# Supplementary material for: Analytical classical density functionals from an equation learning network
Source: arXiv:1910.12752 source file (2019-12-06)
Supplement: Supplementary file 1 [file SI.pdf]

# Supporting Information:
# Analytical classical density functionals from an equation learning network

S.-C. Lin,[1, a)] G. Martius,[2] and M. Oettel[1]
[1)] *Institut für Angewandte Physik, Eberhard Karls Universität Tübingen, 72076 Tübingen, Germany*
[2)] *Max Planck Institute for Intelligent Systems Tübingen, 72076 Tübingen, Germany*

## I. EXACT HARD ROD FUNCTIONAL

The exact form of the excess free energy functional for hard rods (HR) $\mathcal{F}^{\mathrm{HR}}$ is[1,2]

$$\mathcal{F}^{\mathrm{HR}} = \int \phi[n]\, dx = \int -n_0 \ln(1 - n_1)\, dx \tag{1}$$

with $n_i(x) = \rho \otimes \omega_i^{\mathrm{exact}}$ (convolution) , where $\omega_1^{\mathrm{exact}}(x) = \Theta(\sigma/2 - |x|)$ and $\omega_0^{\mathrm{exact}}(x) = \frac{1}{2}\delta(\sigma/2 - |x|)$. Here, $\sigma$ is the length of the rod, $\Theta(x)$ is the Heaviside step function and $\delta(x)$ the Dirac delta function. Thus,

$$\frac{\delta \mathcal{F}^{\mathrm{HR}}}{\delta \rho} = \sum_i \frac{\partial \mathfrak{f}^{\mathrm{HR}}[n]}{\partial n_i} * \omega_i^{\mathrm{exact}}. \tag{2}$$

with $*$ denoting cross-correlation. Eqs. (2) and (1) are used to generate the training profiles in the HR case. In the Lennard–Jones (LJ) case, $\mathcal{F}^{\mathrm{HR}}$ describes the repulsive part of the free energy functional.

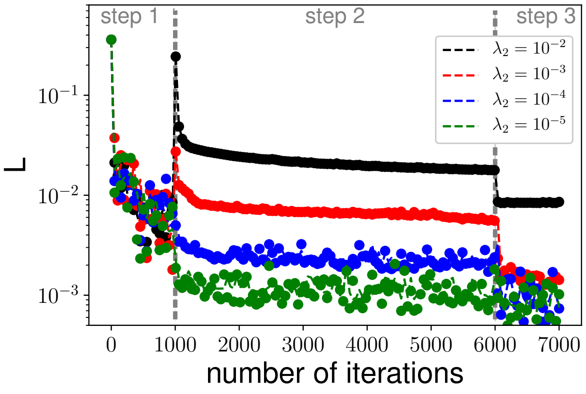


FIG. 1: Loss as a function of number of iterations for 4 different values of $\lambda_2$. Dashed lines are validation loss and solid circles are training loss.

## II. HARD RODS: LEARNING PROCEDURE AND DEPENDENCE ON LOSS FUNCTION PARAMETER $\lambda_2$

In the main paper, we have defined the loss function

$$L = \frac{1}{N}\sum_{i=1}^{N}\left(\alpha_1 \int |\rho_i^{\mathrm{eq}} - \rho_i^{\mathrm{ML}}|\, d\,x + \alpha_2 |\mu_i^{\mathrm{eq}} - \mu_i^{\mathrm{ML}}|\right) + \lambda_1 \sum_i \int dx\, |\omega_i| + \lambda_2 \sum_{l,\beta\gamma} |W_{\beta\gamma}^{(l)}|. \tag{3}$$

The first term quantifies the deviation between generated and input density profile (ground truth) and the corresponding chemical potentials. The second term is is a regularizer to avoid numerically large weight functions during

[a)] Electronic mail: shang-chun.lin@uni-tuebingen.de

the training procedure, and it is not very import for final results. The third term with coefficient $\lambda_2$ is used as a substitute for the number of nonzero entries in the matrices $W^{(l)}$ which is not differentiable directly. Nevertheless minimizing the absolute norm tends to produce sparse solutions, see also Lasso regression[3], and thus favors simpler functionals.

Before training, we prepare 1024 density profiles with a range of reservoir densities $\rho_0 = 0.2...0.55$, and randomly divided into 921 density profiles as training set and 103 as validating set. The training procedure only uses training set for updating trainable parameters and evaluates the value of the loss on the training set and on the validating set (called training loss and validation loss) at the end of each iteration[4]. Additionally, we also prepare 256 density profiles with a range of reservoir densities $\rho_0 = 0.6...0.8$, outside the training region, as a measurement for extrapolative capabilities. Then, as described in the main paper, we have used a three–step training procedure. In Fig. 1 we show the evolution of the training and validation loss throughout the training for 4 different values of $\lambda_2$. For the higher values of $\lambda_2$ ($10^{-2}$ and $10^{-3}$) there is a marked increase of $L$ at the beginning of step 2. For $\lambda = 10^{-4}$ the beginning of step 2 without increase of $L$ and then further decreases.

This is further confirmed in the Fig. 2a, which shows the final value of $L$ from the training, validating, and extrapolating set as a function of $\lambda_2$. The loss shows underfitting for $\lambda_2 > 10^{-3}$ and overfitting for $\lambda_2 < 10^{-7}$. Near–optimal choices are $10^{-6} < \lambda_2 < 10^{-4}$. The complexities (the number of nonzero entries in $W$) increase with decreasing of $\lambda_2$ (Fig. 2b). For a broad range of complexities, the loss is almost constant (Fig. 2c).

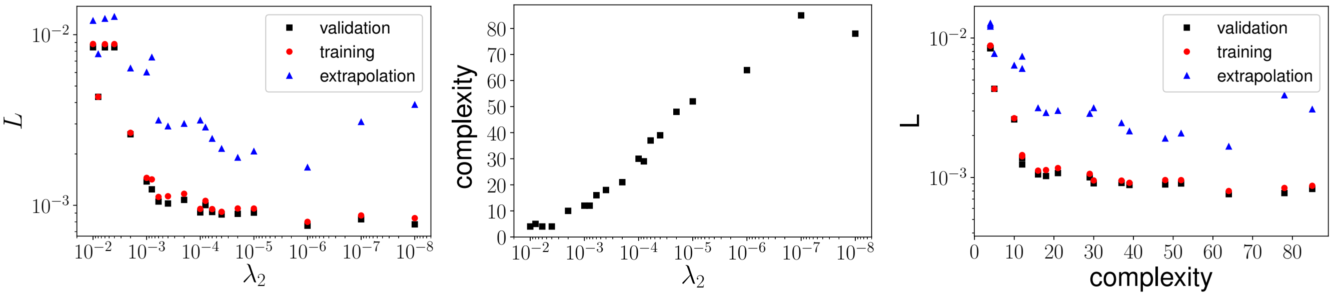


(a) Final loss versus $\lambda_2$.

(b) complexity versus $\lambda_2$.

(c) complexity versus loss.

FIG. 2: The interdependence of loss, complexity and $\lambda_2$.

The effect of $\lambda_2$ on the bulk equation of state (eos) is shown in Fig. 3. The relative deviation of the ML pressure from the exact one (Fig. 3a) is close to zero for $\lambda_2 < 10^{-3}$. In Fig. 3b we analyze the virial coefficients $a_2...a_4$ ($P = \sum_{i=1} a_i \rho^i$, $a_1 = 1$ (ideal gas) and all $a_i = 1$ for the exact eos). Therefore, we finally choose $\lambda_2 = 8 \cdot 10^{-5}$ as a near-optimal compromise between low loss, complexity and eos.

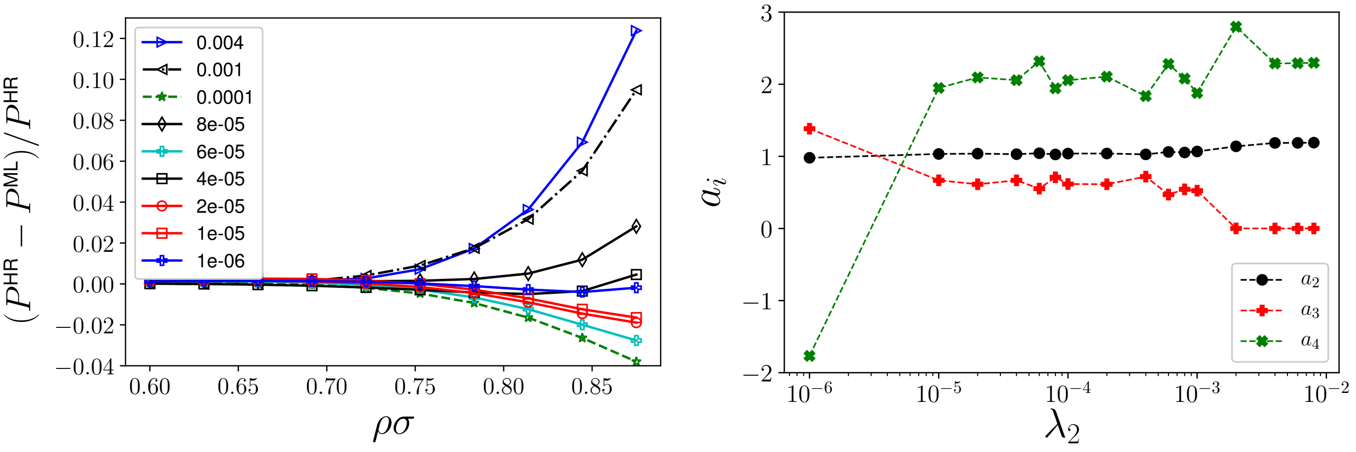


(a) The relative pressure difference as a function of density $\rho$.

(b) Second to fourth virial coefficient as a function of $\lambda_2$.

FIG. 3: Properties of the bulk fluid: pressure and virial coefficients.

## III. CONSISTENCY OF $\mu$

Following Ref. 5, we define $\rho_i^{\rm ML}$ of the $i$–th data set (Eq.(4) in the main paper) by

$$\rho_i^{\rm ML}(x) = \exp\left( \mu_i^{\rm ML} - \frac{\delta \mathcal{F}^{\rm ex,ML}}{\delta \rho}\bigg|_{\rho=\rho_i^{\rm eq}} - V_i^{\rm ext} \right). \qquad (4)$$

Here $\mu_i^{\rm ML}$ is determined by demanding that $\int (\rho_i^{\rm ML} - \rho_i^{\rm eq})^2$ is minimal, which entails that $\mu_i^{\rm ML}$ varies during the iterations. This choice of $\mu_i^{\rm ML}$ stabilizes the training process, and $\mu_i^{\rm ML}$ is directly determined by $\frac{\partial}{\partial \mu_i^{\rm ML}} \int (\rho_i^{\rm ML} - \rho_i^{\rm eq})^2 = 0$ $\Rightarrow \mu_i^{\rm ML} = \ln\left( \frac{\int \rho_i^{\rm eq} \rho_i'^{\,\rm ML}}{\int (\rho_i'^{\,\rm ML})^2} \right)$, where $\rho_i'^{\,\rm ML} = \exp\left( -\frac{\delta \mathcal{F}^{\rm ex,ML}}{\delta \rho}\bigg|_{\rho=\rho_i^{\rm eq}} - V_i^{\rm ext} \right)$. If the training converges, $\mu^{\rm ML}$ will converge to $\mu^{\rm eq}$. In Fig.4 we show $\Delta\mu = \mu^{\rm eq} - \mu^{\rm ML}$ versus $\mu^{\rm eq}$ at the end of training for the three cases in the main paper, and $\mu^{\rm ML}$ is indeed close to $\mu^{\rm eq}$.

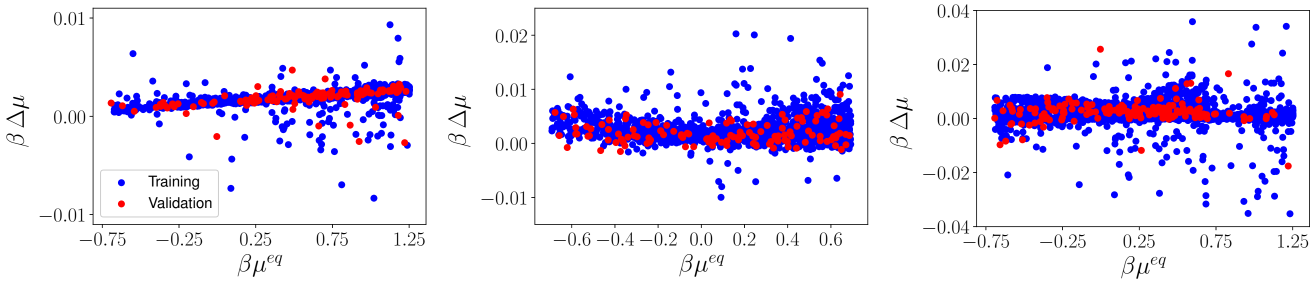


(a) HR (b) LJ with splitting (c) LJ, no splitting

FIG. 4: $\Delta\mu = \mu^{\rm eq} - \mu^{\rm ML}$ versus $\mu^{\rm eq}$. (a) HR (b) LJ with splitting (c) LJ, no splitting.

Furthermore, we also check $\mu(\rho) = \frac{\partial \mathfrak{f}}{\partial \rho}$ (i.e. from the equation of state), where $\rho$ here refers to the density of the bulk fluid. In Fig. 5 we show $\mu(\rho)$ by exact functional, ML, and MC simulations for the three cases as in the main paper. Deviations only occur for the LJ case well outside the training region.

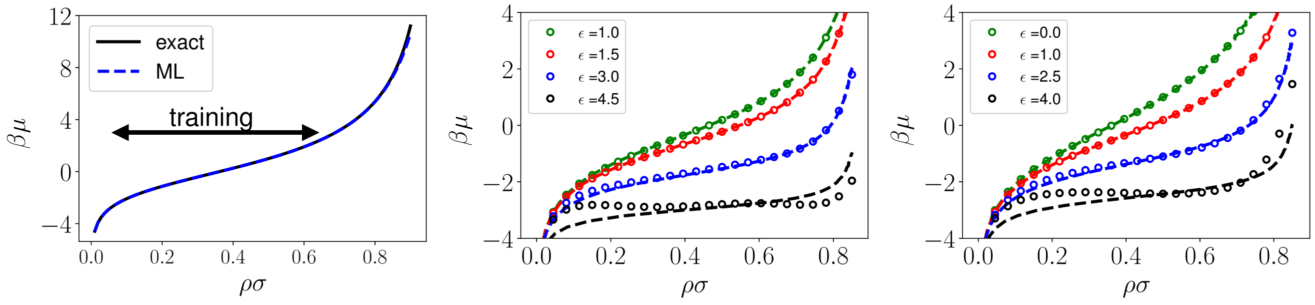


(a) HR (b) LJ with splitting (c) LJ, no splitting

FIG. 5: $\mu(\rho)$ versus $\rho$. (a) HR (b) LJ with splitting (c) LJ, no splitting. In (b) and (c), the circles are ML and dashed lines are MC simulations.

In principle, one could also fix $\mu_i^{\mathrm{ML}} = \mu_i^{\mathrm{eq}}$ (the chemical potential of the data set) and then choose $\alpha_1 = 1$ and $\alpha_2 = 0$ in Eq. (3), but this requires smaller learning rates and results in much longer training processes. For example, the HR case with parameters as in the main paper can be done with learning rate $= 10^{-3}$ and the number of training iterations doubled.

## IV. COMPARISON AMONG $\mathcal{F}^{\mathrm{ex,ML}}$ FOR LJ FLUID

In Ref. 5, the $\mathcal{F}^{\mathrm{ex,ML}}$ is limit to the polynomial *ansatz* and the best one is given by

$$\mathcal{F}^{\mathrm{ex,ML}}_{o=3} = \mathcal{F}^{\mathrm{HR}} + \epsilon \left( \int dx \sum_{ij} \beta_{ij} n_i n_j + \sum_{i,j,k} \gamma_{ijk} n'_i n'_j n'_k \right) \tag{5}$$

with $i, j, k$ run from 0 to 7, thus we have 16 weighted densities in total. In Fig. 6 we show the equation of state $P(\rho)$ with $\epsilon = 2.5$ and $\rho(x)$ with $\epsilon = 1.7$ and $\mu = \ln(1.7)$ at a hard wall. Both results show that FEQL is better then the polynomial *ansatz* in Ref. 5.

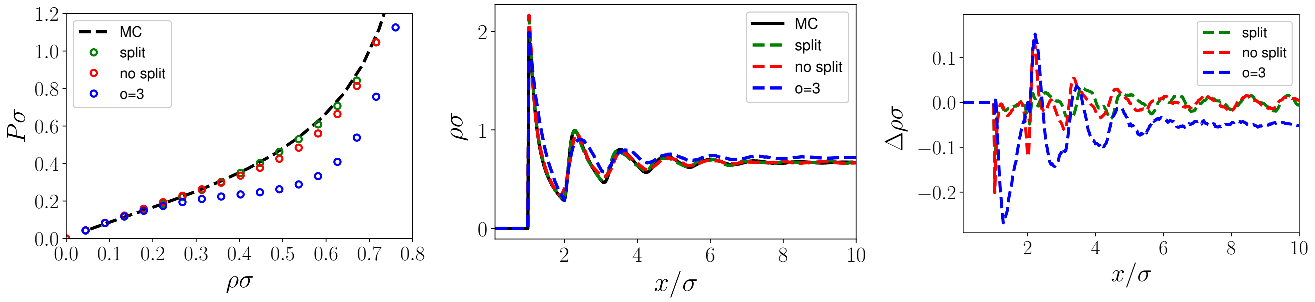


(a) $P(\rho)$ (b) $\rho(x)$ at a hard wall (c) $\Delta\rho(x)$ at a hard wall

FIG. 6: Comparison among three $\mathcal{F}^{\mathrm{ex,ML}}$ for LJ fluid, two from the main paper and $\mathcal{F}^{\mathrm{ex,ML}}_{o=3}$ from Ref. 5. (a) $P(\rho)$ with $\epsilon = 2.5$. (b) $\rho(x)$ at a hard wall with $\epsilon = 1.7$ and $\mu = \ln(1.7)$. (c) $\Delta\rho(x) = \rho^{\mathrm{MC}}(x) - \rho^{\mathrm{ML}}(x)$ with the same condition as (b). Note that the training data are $\epsilon = 1.0...1.5$ for $\mathcal{F}^{\mathrm{ex,ML}}_{o=3}$ and $\epsilon = 0.5...1.5$ for two $\mathcal{F}^{\mathrm{ex,ML}}$ form the main paper.

## V. FULL $\mathcal{F}^{\mathrm{ex,ML}}$

Here we show the full functional of $\mathcal{F}^{\mathrm{ex,ML}}[n]$, with $n_i(x) = \int dx' \rho(x')\omega_i(x - x')$. The coefficients in $\mathcal{F}^{\mathrm{ex,ML}}$ are single precision; for displaying purposes, all coefficients are rounded to the one decimal place and then rationalized. For $\mathcal{F}^{\mathrm{ex,ML}}$ with full digits, we provide `test_function.ipynb` (*Jupyter notebook*). Also, in `test_function.ipynb` and other notebooks, we demonstrate how to use trained functional to obtain equilibrium density profiles, eos, and direct correlation function[6].

### A. $\mathcal{F}^{\mathrm{ex,ML}}$ for hard rod

The FEQL result for hard rod is

$$\mathcal{F}^{\mathrm{ex,ML}} = \int dx \, \frac{\frac{n_0^2}{5} + \frac{n_0}{10} y_0 - \frac{n_2^2}{10}}{-\frac{n_0^2}{5} - \frac{n_0}{5} y_0 - \frac{n_0}{10} + \frac{e^{y_1}}{5} + \frac{4}{5}} + y_2 \left( -\frac{n_0^2}{5} - \frac{n_0}{10} y_0 - \frac{3}{10} e^{y_1} + \frac{3}{10} \right) + e^{y_3} - 1 \tag{6}$$

with $y_0 = \frac{2n_0}{5} + \frac{n_2}{5}$, $y_1 = \frac{3n_1}{5}$, $y_2 = \frac{2n_0}{5} - \frac{n_1}{5} + \frac{n_2^2}{10} - \frac{n_2}{10}$, $y_3 = \frac{n_0^2}{10}$ and convolution kernels $\omega_i$ shown in Fig.7a.

### B. $\mathcal{F}^{\text{ex,ML}}$ for LJ with splitting

$\mathcal{F}^{\text{ex}} = \mathcal{F}^{\text{HR}} + \epsilon\mathcal{F}^{\text{ex,ML}}_{\text{att}}$, where

$$\mathcal{F}^{\text{ex,ML}}_{\text{att}} = \int dx\, \frac{3}{5}y_0y_1\left(-\frac{\epsilon n_3}{2} - \frac{n_0}{10} - \frac{n_1}{10} - \frac{n_2}{2} + \frac{y_0y_1}{5} - \frac{y_2y_3}{5} - \frac{2y_4}{5y_5}\right) - \frac{y_0y_1}{10} - \frac{y_2y_3}{5}$$
$$- \frac{y_2y_3}{10\left(\frac{\epsilon n_3}{5} + \frac{n_2}{5} - \frac{7y_0y_1}{10} + \frac{3y_2y_3}{5} - \frac{2\ln y_6}{5} + 1 - \frac{-\epsilon n_3 - \frac{n_0}{2} - \frac{n_1}{10} - \frac{11n_2}{10}}{10y_5}\right)}$$
$$+ \left(\frac{3\epsilon n_3}{10} + \frac{n_0}{10} + \frac{3n_2}{10} - \frac{y_0y_1}{2} + \frac{9y_2y_3}{10} + \frac{\ln y_6}{10} + \frac{-\epsilon n_3 - \frac{n_0}{2} - \frac{n_1}{10} - \frac{11n_2}{10}}{10y_5}\right)$$
$$\left(-\frac{3\epsilon n_3}{10} - \frac{n_0}{10} - \frac{n_1}{10} - \frac{2n_2}{5} + \frac{3y_0y_1}{10} - \frac{3y_2y_3}{10} + \frac{e^{y_7}}{5} - \frac{1}{5} - \frac{9y_4}{10y_5}\right) + e^{-\frac{2y_0y_1}{5} - \frac{y_2y_3}{5}} + \ln\left(-\frac{y_2y_3}{5} + 1\right) - 1 \tag{7}$$

with

$$y_0 = \frac{n_0}{5} - \frac{2n_1}{5} + \frac{n_2}{10},\ y_1 = \frac{\epsilon n_3}{2} - \frac{3n_0}{10} - \frac{2n_1}{5} + \frac{3n_2}{10},\ y_2 = \frac{\epsilon n_3}{10} + \frac{n_0}{5} - \frac{3n_1}{10} - \frac{2n_2}{5},\ y_3 = \frac{\epsilon n_3}{10} + \frac{n_0}{5} + \frac{n_1}{5} - \frac{3n_2}{10},$$
$$y_4 = -\epsilon n_3 - \frac{n_0}{2} - \frac{n_1}{10} - \frac{11n_2}{10},\ y_5 = -\frac{2\epsilon n_3}{5} - \frac{6n_1}{5} + 1,\ y_6 = -\frac{3\epsilon n_3}{10} + \frac{n_2}{10} + 1,\ y_7 = -\frac{\epsilon n_3}{5} + \frac{2n_0}{5}$$

and convolution kernels $\omega_i$ shown in Fig.7b

### C. $\mathcal{F}^{\text{ex,ML}}$ for LJ without splitting

The result of $\mathcal{F}^{\text{ex}}$ given by FEQL is

$$\mathcal{F}^{\text{ex,ML}} = \int dx\, \frac{y_0\ln y_1}{10} + \frac{y_2y_3}{10} + \frac{-\frac{y_4y_5}{2} + \frac{3y_2y_3}{10} - \frac{y_6y_7}{2}}{\frac{3y_4y_5}{10} + \frac{3\ln y_1}{10} + 1} + \left(-\frac{y_4y_5}{5} + \frac{17e^{y_8}}{10} + \frac{4\ln y_1}{5} - \frac{17}{10}\right)$$
$$\left(-\frac{3\epsilon n_3}{5} - \frac{n_0}{10} + \frac{n_2}{5} + \frac{y_2y_3}{2} - \frac{9\ln y_1}{5}\right) + \left(-\frac{\epsilon n_3}{5} + \frac{n_2}{10} + \frac{3y_4y_5}{10} + \frac{-\frac{n_0}{10} - \frac{n_1}{5} + \frac{n_2}{10}}{5y_9} + \frac{y_6y_7}{5}\right)$$
$$\left(-\frac{\epsilon n_3}{5} + \frac{n_2}{10} + \frac{2y_4y_5}{5} + \frac{-\frac{n_0}{10} - \frac{n_1}{5} + \frac{n_2}{10}}{5y_9} + \frac{y_6y_7}{5} + \frac{e^{y_8}}{10} - \frac{1}{10}\right)$$
$$+ e^{\frac{y_2y_3}{5} - \frac{3y_6y_7}{10}} + \ln\left(\frac{y_2y_3}{10} + 1\right) - 1 \tag{8}$$

with

$$y_0 = -\frac{\epsilon n_3}{5} + \frac{n_2}{10},\ y_1 = -\frac{7n_1}{10} - \frac{7n_2}{10} + 1,\ y_2 = \frac{3\epsilon n_5}{10} - \frac{2n_0}{5} + \frac{n_2}{10},\ y_3 = \frac{2\epsilon n_4}{5} - \frac{2\epsilon n_5}{5} - \frac{n_1}{10} - \frac{n_2}{10},$$
$$y_4 = -\frac{3n_0}{10} - \frac{n_1}{2} + \frac{3n_2}{10},\ y_5 = \frac{2n_0}{5} + \frac{2n_1}{5} - \frac{3n_2}{10},\ y_6 = -\frac{\epsilon n_5}{5} - \frac{3n_0}{10} - \frac{2n_1}{5} + \frac{3n_2}{10},$$
$$y_7 = \frac{\epsilon n_5}{2} + \frac{n_0}{10} + \frac{2n_1}{5} - \frac{n_2}{5},\ y_8 = \frac{n_0}{10} - \frac{3n_1}{10} - \frac{3n_2}{5},\ y_9 = -\frac{3n_0}{10} - \frac{n_1}{2} + \frac{n_2}{10} + 1$$

and convolution kernels $\omega_i$ shown in Fig.7c

## VI. FEQL BUILDING AND PHYSICAL CONSTRAINTS

To build FEQL, we first use *SymPy*[7] to determine $\mathcal{F}^{\text{ex,ML}}$ and $\frac{\partial \mathfrak{f}^{\text{ex,ML}}}{\partial n_i}$ with a given number of weighted densities $n_{\text{w}}$, levels and nodes. Second, we feed the $\frac{\partial \mathfrak{f}^{\text{ex,ML}}}{\partial n_i}$ and trainable parameters into *Tensorflow*[8]; then add other layers to fit the DFT structure (convolutions and Eq.(4) in the main paper). Finally, the network is trained by *Keras*[9] with *Tensorflow* backend.

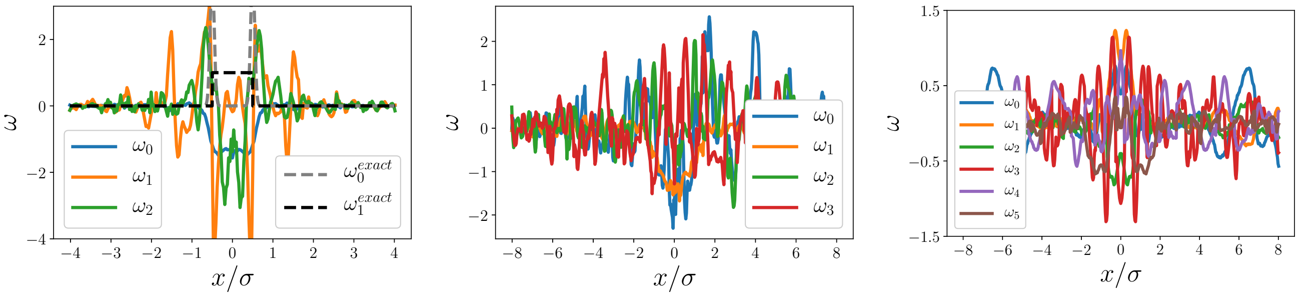


(a) $\omega^{\mathrm{HR}}$ for Eq.(6) (b) $\omega^{\mathrm{LJ}}$ for Eq.(7) (c) $\omega^{\mathrm{LJ}}$ for Eq.(8)

FIG. 7: $\omega$ for all cases. (a)HR. The $\omega_i^{\mathrm{exact}}$ are the exact weighting kernels in Eqs. (1) and (2). (b)LJ, splitting (c)LJ, no splitting. The maximum allowed range for the kernels is $[-4\sigma, 4\sigma]$ in the HR case and $[-8\sigma, 8\sigma]$ in the LJ case.

Since $\mathcal{F}^{\mathrm{ex,ML}}$ approximates $\mathcal{F}^{\mathrm{ex}}$, we must consider two physical constraints: (i) $\mathcal{F}^{\mathrm{ex,ML}}(\rho = 0) = 0$ and (ii) $\left.\frac{\delta\mathcal{F}^{\mathrm{ex,ML}}}{\delta\rho}\right|_{\rho=0} = 0$. To enforce (i), we choose the linear mapping without bias and $f(0) = g(0,z) = 0$ in the non–linear mapping. Condition (ii) can be enforced by setting appropriate parameters form the matrix $W^{(l)}$ of the final level to zero. This requires to determine the analytic form of $\left.\frac{\partial\mathfrak{f}^{\mathrm{ex,ML}}}{\partial n_i}\right|_{\rho=0}$ to identity those parameters. For example, for a FEQL with $n_{\mathrm{w}} = 2$, 2 levels and (1,1,1,1,1) nodes nodes for (identity, exponential, logarithm, multiplication and division),

$$
\begin{aligned}
\mathfrak{f}^{\mathrm{ex,ML}} =\ & a_2L_0\left(a_1L_0n_0 + a_1L_1n_1\right) + a_2L_1\left(e^{a_1L_2n_0 + a_1L_3n_1} - 1\right) + a_2L_2 \ln\left(a_1L_4n_0 + a_1L_5n_1 + 1\right) + a_2L_3\left(a_1L_6n_0 + a_1L_7n_1\right)\left(a_1L_8n_0 + a_1L_9n_1\right) \\
& + \frac{a_2L_4\left(a_1L_{10}n_0 + a_1L_{11}n_1\right)}{a_1L_{12}n_0 + a_1L_{13}n_1 + 1} + \Big(a_2L_{15}\left(a_1L_0n_0 + a_1L_1n_1\right) + a_2L_{16}\left(e^{a_1L_2n_0 + a_1L_3n_1} - 1\right) + a_2L_{17}\ln\left(a_1L_4n_0 + a_1L_5n_1 + 1\right) + \\
& a_2L_{18}\left(a_1L_6n_0 + a_1L_7n_1\right)\left(a_1L_8n_0 + a_1L_9n_1\right) + \frac{a_2L_{19}\left(a_1L_{10}n_0 + a_1L_{11}n_1\right)}{a_1L_{12}n_0 + a_1L_{13}n_1 + 1}\Big)\Big(a_2L_{20}\left(a_1L_0n_0 + a_1L_1n_1\right) + a_2L_{21}\left(e^{a_1L_2n_0 + a_1L_3n_1} - 1\right) \\
& + a_2L_{22}\ln\left(a_1L_4n_0 + a_1L_5n_1 + 1\right) + a_2L_{23}\left(a_1L_6n_0 + a_1L_7n_1\right)\left(a_1L_8n_0 + a_1L_9n_1\right) + \frac{a_2L_{24}\left(a_1L_{10}n_0 + a_1L_{11}n_1\right)}{a_1L_{12}n_0 + a_1L_{13}n_1 + 1}\Big) + \\
& \Big(a_2L_{25}\left(a_1L_0n_0 + a_1L_1n_1\right) + a_2L_{26}\left(e^{a_1L_2n_0 + a_1L_3n_1} - 1\right) + a_2L_{27}\ln\left(a_1L_4n_0 + a_1L_5n_1 + 1\right) + a_2L_{28}\left(a_1L_6n_0 + a_1L_7n_1\right) \\
& \left(a_1L_8n_0 + a_1L_9n_1\right) + \frac{a_2L_{29}\left(a_1L_{10}n_0 + a_1L_{11}n_1\right)}{a_1L_{12}n_0 + a_1L_{13}n_1 + 1}\Big) \Big/ \Big(a_2L_{30}\left(a_1L_0n_0 + a_1L_1n_1\right) + a_2L_{31}\left(e^{a_1L_2n_0 + a_1L_3n_1} - 1\right) + \\
& a_2L_{32}\ln\left(a_1L_4n_0 + a_1L_5n_1 + 1\right) + a_2L_{33}\left(a_1L_6n_0 + a_1L_7n_1\right)\left(a_1L_8n_0 + a_1L_9n_1\right) + \frac{a_2L_{34}\left(a_1L_{10}n_0 + a_1L_{11}n_1\right)}{a_1L_{12}n_0 + a_1L_{13}n_1 + 1} + 1\Big) + \\
& e^{a_2L_5\left(a_1L_0n_0 + a_1L_1n_1\right) + a_2L_6\left(e^{a_1L_2n_0 + a_1L_3n_1} - 1\right) + a_2L_7\ln\left(a_1L_4n_0 + a_1L_5n_1 + 1\right) + a_2L_8\left(a_1L_6n_0 + a_1L_7n_1\right)\left(a_1L_8n_0 + a_1L_9n_1\right) + \frac{a_2L_9\left(a_1L_{10}n_0 + a_1L_{11}n_1\right)}{a_1L_{12}n_0 + a_1L_{13}n_1 + 1}} \\
& + \ln\Big(a_2L_{10}\left(a_1L_0n_0 + a_1L_1n_1\right) + a_2L_{11}\left(e^{a_1L_2n_0 + a_1L_3n_1} - 1\right) + a_2L_{12}\ln\left(a_1L_4n_0 + a_1L_5n_1 + 1\right) + \\
& a_2L_{13}\left(a_1L_6n_0 + a_1L_7n_1\right)\left(a_1L_8n_0 + a_1L_9n_1\right) + \frac{a_2L_{14}\left(a_1L_{10}n_0 + a_1L_{11}n_1\right)}{a_1L_{12}n_0 + a_1L_{13}n_1 + 1} + 1\Big) - 1
\end{aligned}
$$

with $a_xL_y$ the $y$–th parameter in $W^{(x)}$. Then we calculate $\left.\frac{\partial\mathfrak{f}^{\mathrm{ex,ML}}}{\partial n_i}\right|_{\rho=0}$, such as

$$
\begin{aligned}
\left.\frac{\partial\mathfrak{f}^{\mathrm{ex,ML}}}{\partial n_0}\right|_{\rho=0} =\ & a_1L_0a_2L_0 + a_1L_0a_2L_{10} + a_1L_0a_2L_{25} + a_1L_0a_2L_5 + a_1L_{10}a_2L_{14} + a_1L_{10}a_2L_{29} + a_1L_{10}a_2L_4 + a_1L_{10}a_2L_9 \\
& + a_1L_2a_2L_1 + a_1L_2a_2L_{11} + a_1L_2a_2L_{26} + a_1L_2a_2L_6 + a_1L_4a_2L_{12} + a_1L_4a_2L_2 + a_1L_4a_2L_{27} + a_1L_4a_2L_7
\end{aligned}
$$

and

$$
\begin{aligned}
\left.\frac{\partial\mathfrak{f}^{\mathrm{ex,ML}}}{\partial n_1}\right|_{\rho=0} =\ & a_1L_1a_2L_0 + a_1L_1a_2L_{10} + a_1L_1a_2L_{25} + a_1L_1a_2L_5 + a_1L_{11}a_2L_{14} + a_1L_{11}a_2L_{29} + a_1L_{11}a_2L_4 + a_1L_{11}a_2L_9 \\
& + a_1L_3a_2L_1 + a_1L_3a_2L_{11} + a_1L_3a_2L_{26} + a_1L_3a_2L_6 + a_1L_5a_2L_{12} + a_1L_5a_2L_2 + a_1L_5a_2L_{27} + a_1L_5a_2L_7
\end{aligned}
$$

Thus we set $a_2L_{11}$, $a_2L_{29}$, $a_2L_2$, $a_2L_{26}$, $a_2L_{25}$, $a_2L_9$, $a_2L_{12}$, $a_2L_7$, $a_2L_{27}$, $a_2L_5$, $a_2L_4$, $a_2L_{10}$, $a_2L_{14}$, $a_2L_1$, $a_2L_6$ and $a_2L_0$ to zero in order to keep $\left.\frac{\delta\mathcal{F}^{\mathrm{ex,ML}}}{\delta\rho}\right|_{\rho=0} = 0$.

[1] J. K. Percus, J. Stat. Phys. **15**, 505 (1976).
[2] Y. Rosenfeld, M. Schmidt, H. Löwen, and P. Tarazona, Physical Review E **55**, 4245 (1997).
[3] R. Tibshirani, J. R. Stat. Soc. Series B Stat. Methodol. , 267 (1996).
[4] P. Mehta, M. Bukov, C.-H. Wang, A. G. Day, C. Richardson, C. K. Fisher, and D. J. Schwab, Phys. Rep. (2019).
[5] S.-C. Lin and M. Oettel, SciPost Phys. **6**, 025 (2019).
[6] S.-C. Lin, "FEQL," `https://github.com/ShangChunLin/FEQL` (2019).
[7] Meurer *et al.*, PeerJ Comput. Sci. **3**, e103 (2017).
[8] M. Abadi *et al.*, "TensorFlow: Large-scale machine learning on heterogeneous systems," (2015), software available from tensorflow.org.
[9] F. Chollet *et al.*, "Keras," `https://keras.io` (2015).
